# Supplementary material for: Termination of lambda-calculus with the extra Call-By-Value rule known as assoc
Source: arXiv:0806.4859 source file (2008-09-02)
Supplement: Supplementary file 1 [file Appendix2.tex]

\section{Examples}
\begin{example}
We give examples of unwanted reductions (leading to non-termination),
which motivated the side-conditions of two rules of \lLJQ.

Suppose that $W$ is an abstraction and $N$ is a $y$-covalue.
The reductions\linebreak $\letin{\letin {\cst W} y N} z P\Rew{}\letin {\cst W} y
{\letin{N} z P}$ and $\letin {\cst W} y N\Rew{}\JCrx {\cst W} y N$ are
not valid (as the side-conditions of the rules are not satisfied).
Our first-order encoding
translates them to
$$
\begin{array}{lll}
{\subi[(\l y.\ql P)\ {\subst{\ql N}y{\ql W}}]
{\subi[{\subst{\ql N}y{\ql W}}]{\un{\foc W}}{\foc N}}
{\foc P}}& \not\!\!\!\glpo& \subiii[\subst{((\l z.\ql {P})\ \ql {N})}y
{\ql W}]{\un{\foc W}}{\subiii[(\l z.\ql {P})\ \ql
{N}]{\foc {N}} {\foc {P}}}\\\\
\subi[{\subst{\ql N}y{\ql W}}]{\un{{\foc W}}}{\foc N}
&\not\!\!\!\glpo& \subii[\subst{\ql
{N}}y{\ql {W}}]{\foc W}{\foc {N}}
\end{array}
$$ Indeed, non-termination of these reductions can be seen as we can
turn $\letin {\ }{\ }{\ }$ into $\JCrx {\ }{\ }{\ }$ and back:
$$
\begin{array}{c}
\letin{\letin {\cst {W}} y {{N}}} z {P}\\
\begin{array}{cc}
\swarrow&\searrow\\
\letin {\cst {W}} y {\letin{{N}} z {P}}
&\letin{\JCrx {{W}} y {{N}}} z {P}\\
\downarrow&\downarrow\\
\JCrx {W} y {\letin{N} z {P}}
&\letin{\letin {\cst{W}} y {N'}} z {P}\\
\downarrow\\
\letin{\JCrx {W} y {N}} z {P'}\\
\downarrow\\
\letin{\letin {\cst{W}} y {N'}} z {P'}
\end{array}
\end{array}
$$ where $P'=\JCrx {W} y {P}$ (but note that $y\not\in\FV {P}$) and
$N'$ is the $y$-covalue obtained by pushing $W$ inside the $y$-covalue
$N$.
\end{example}

\newpage\begin{example}
On the other hand, the following reductions {\emph {are}} allowed (under which
the image by $\ql{(\ \cdot\ )}$ is unchanged).

$$
\begin{array}{c}
\JCrx V x{\letin{\letin {\cst W} y N} z P}\\
\downarrow_+\\
\letin{\letin {\cst {W'}} y {\JCrx V x{N}}} z {P'}\\
\begin{array}{cc}
\swarrow&\searrow\\
\letin {\cst {W'}} y {\letin{\JCrx V x{N}} z {P'}}
&\letin{\JCrx {{W'}} y {\JCrx V x{N}}} z {P'}\\
\downarrow&\downarrow\\
\letin {\cst {W'}} y {\letin{N'} z {P'}}
&\letin{\JCrx {{W'}} y {N'}} z {P'}\\
\downarrow&\downarrow\\
\JCrx {W'} y {\letin{N'} z {P'}}
&\letin{\letin {\cst{W'}} y {N''}} z {P'}\\
\downarrow\\
\letin{\JCrx {W'} y {N'}} z {P''}\\
\downarrow\\
\letin{\letin {\cst{W'}} y {N''}} z {P''}
\end{array}
\end{array}
$$ where $W'=\JCrx V x W$, $P'=\JCrx V x P$, $P''=\JCrx {W'} y {P'}$
(but note that $y\not\in\FV {P'}$), $N'$ is the $y$-covalue obtained
by pushing $V$ inside the $y$-covalue $N$, and $N''$ is the
$y$-covalue obtained by pushing $W'$ inside the $y$-covalue $N'$.

This motivated the case distinctions leading to
$\subiname,\subiiname,\subiiiname$ and $\subivname$ and their
precedence. Indeed we have
$$
\begin{array}{ll}
&\subiv [\subst{((\l z.\ql P)\ {\subst{\ql N}y{\ql W}})}x{\ql V}]{\foc V}{\subi[(\l y.\ql P)\ {\subst{\ql N}y{\ql W}}]{\subi[{\subst{\ql N}y{\ql W}}]{\un{\foc W}}{\foc N}} {\foc P}}\\
\glpo&\subiii[(\l z.\ql {P'})\ \subst{\subst{\ql N}x{\ql V}}y{\ql {W'}}]{\subiii[\subst{\subst{\ql N}x{\ql V}}y{\ql {W'}}]{\un{\foc {W'}}}{\subiv[\subst{N}x{\ql V}] {\foc V}{\foc N}}} {\foc {P'}}
\end{array}
$$
In the first branch we then get
$$
\begin{array}{ll}
\glpo&\subiii[\subst{((\l z.\ql {P'})\ \subst{\ql N}x{\ql V})}y
{\ql {W'}}]{\un{\foc{W'}}}{\subiii[(\l z.\ql {P'})\ \subst{\ql N}x{\ql V}]{\subiv[\subst{N}x{\ql V}] {\foc V}{\foc N}} {\foc {P'}}}\\
\glpo&\subiii[\subst{((\l z.\ql {P'})\ {\ql {N'}})}y
{\ql {W'}}]{\un{\foc{W'}}}{\subiii[(\l z.\ql {P'})\ {\ql {N'}}]{\foc {N'}} {\foc {P'}}}\\
\glpo&\subii[\subst{((\l z.\ql {P'})\ {\ql {N'}})}y
{\ql {W'}}]{{\foc{W'}}}{\subiii[(\l z.\ql {P'})\ {\ql {N'}}]{\foc {N'}} {\foc {P'}}}\\
\glpo&\subi[(\l z.\ql {P''})\ \subst{\ql {N'}}y
{\ql {W'}}]{\subii[\subst{\ql {N'}}y
{\ql {W'}}]{\foc{W'}}{\foc {N'}}} {\foc {P''}}\\
\glpo&\subi[(\l z.\ql {P''})\ \subst{\ql {N''}}y
{\ql {W'}}]{\subi[\subst{\ql {N''}}y
{\ql {W'}}]{\un{\foc{W'}}}{\foc {N''}}} {\foc {P''}}\\
\end{array}
$$
In the second branch we then get
$$
\begin{array}{ll}
\glpo&\subiii[(\l z.\ql {P'})\ \subst{\subst{\ql N}x{\ql V}}y{\ql
  {W'}}]{\subii[\subst{\subst{\ql N}x{\ql V}}y{\ql {W'}}]{{\foc
      {W'}}}{\subiv[\subst{N}x{\ql V}] {\foc V}{\foc N}}} {\foc
  {P'}}\\
\glpo&\subiii[(\l z.\ql {P'})\ \subst{\ql {N'}}y{\ql {W'}}]{\subii[\subst{\ql {N'}}y{\ql {W'}}]{{\foc {W'}}}{\foc {N'}}} {\foc {P'}}\\
\glpo&\subiii[(\l z.\ql {P'})\ \subst{\ql {N''}}y{\ql {W'}}]{\subi[\subst{\ql {N''}}y{\ql {W'}}]{\un{\foc {W'}}}{\foc {N'}}} {\foc {P'}}\\
\end{array}
$$

In this example, we performed reductions dangerously close to the
forbidden ones above (destroying or activating the principal cut), and
both branches look like loops that turn $\letin {\ }{\ }{\ }$ into
$\JCrx {\ }{\ }{\ }$ and back, except that this time, we have consumed
$V$ along the way.

Indeed, the first-order terms we have produced along the reductions
are rather big (note the $\subiiiname$-constructs) in comparison to
$\subi[(\l y.\ql P)\ {\subst{\ql N}y{\ql W}}]{\subi[{\subst{\ql
N}y{\ql W}}]{\un{\foc W}}{\foc N}} {\foc P}$, but in fact they are
never compared against it but against the $\subivname$-construct of
$\JCrx V x{}$. In other words, we have been able to perform this
dangerous reductions only at the cost of pushing $V$ in, and such
things to push are not in infinite supplies.
\end{example}
